# Supplementary material for: Transition of Social Organisations Driven by Gift Relationship
Source: arXiv:2205.11133 source file (2022-06-08)
Supplement: Supplementary file 1 [file gift_si.pdf]

# Supplementary Information for “Transition of Social Organisations Driven by Gift Relationship”

KENJI ITAO<sup>1</sup> AND KUNIHICO KANEKO<sup>\*</sup>

<sup>\*</sup>kaneko@complex.c.u-tokyo.ac.jp

## SUPPLEMENTARY FIGURE

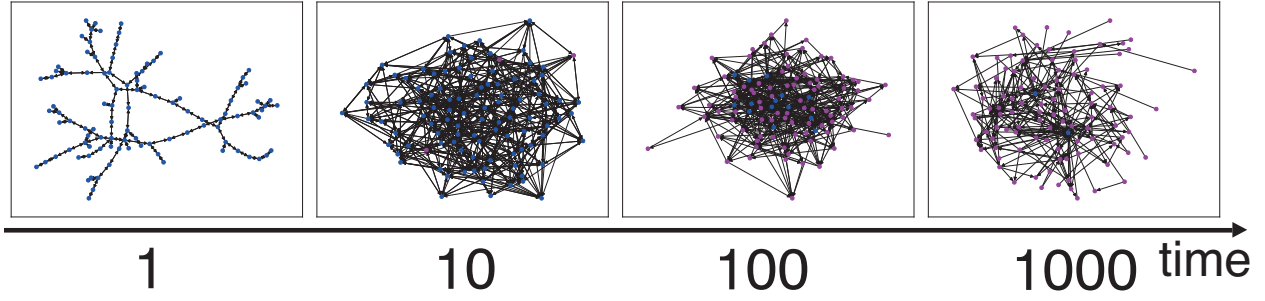

**Figure S1.** Temporal change of network structure in the basic model. Edges with the weights larger than  $\eta$  are shown. Red nodes represent the “repaying” people who are in the process of repayment. Blue nodes represent the “free” people who are not in that process. As time passes, that is, many gifts are exchanged, the network is denser and subsequently, edges are concentrated on a few people. However, no clusters are observed in the beginning, since we do not consider kin relations, as compared with Fig.3.

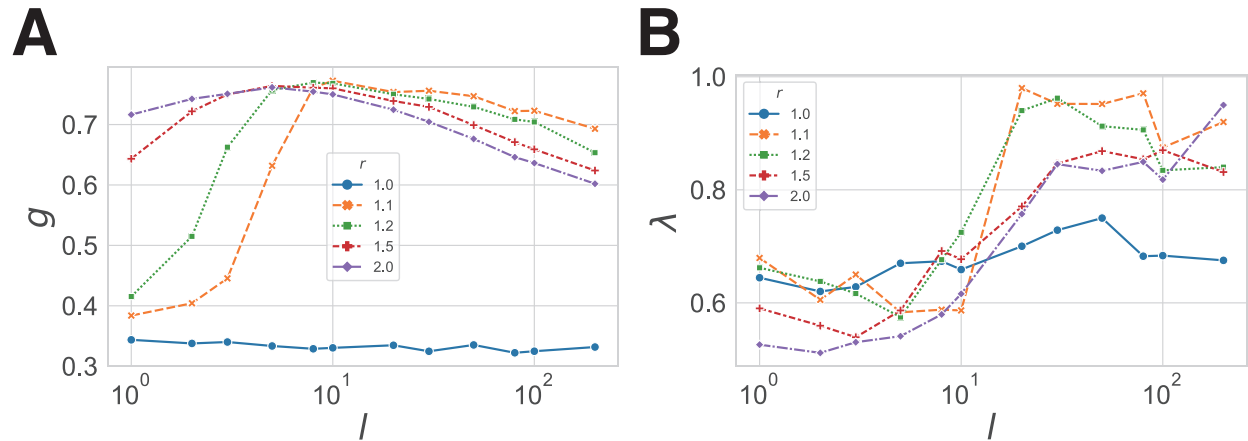

**Figure S2.** Evolution of strategies for the ratio of wealth spent on the gift (A) and the inequality in the inheritance (B). These strategy values are transmitted from parents to children with slight mutations. Figures show the average of each strategy value after  $300l$  steps. (A) The ratio of wealth spent on the gift  $g$ . Each time, the individual  $i$  gives  $g_i w_i$  of wealth as a gift. As long as  $r \geq 1$ ,  $g > 0$  and gifts are certainly exchanged. Furthermore, a considerable ratio of wealth is donated as a gift under sufficiently large  $l$  and  $r$ . (B) The inequality in inheritance  $\lambda$  is defined as follows: Let the individual  $i$  has  $N_i$  children. The  $j$ th child inherits  $\exp(-\lambda_i j) / \sum_{k=0}^{N_i} \exp(-\lambda_i k)$  of wealth and connectivity from the parent.  $\lambda = 0$  corresponds to the equal inheritance, whereas a larger  $\lambda$  corresponds to the exclusive inheritance. When  $r = 1$ ,  $\lambda$  is almost independent of  $l$  and exhibits the moderate inequality in the inheritance. When  $r > 1$ , however, it is small and equal inheritance evolves for small  $l$ , whereas it is large and exclusive inheritance evolves for large  $l$ . This transition in the inheritance inequality occurs together with the rise of the economic disparity in Fig. 2.

## SUPPLEMENTARY TABLES

**Table S1.** Correlation of cultural and environmental characteristics with the gift degree. Using the data of 155 societies, we calculated Spearman's rank correlations between the SCCS variables and the estimated gift degree. This table presents the variables that exhibited high correlation. A larger value for each variable indicates that the item is observed to a greater degree in societies (e.g. a large value for SCCS571 shows that the society is rich in resources.). SCCS 571, SCCS 1463, SCCS1130, SCCS1122, and SCCS1565 suggest that the gift degree is large in larger populations and herding societies, whereas it is small in hunting societies. SCCS711, SCCS835, SCCS158, SCCS237, SCCS1740, and SCCS699 suggest that societies are hierarchically organised when the gift degree is large. SCCS883, SCCS884, SCCS706, SCCS153, and SCCS756 suggest that the specialisation of people increases as the gift degree is larger.

| Name     | Explanation                                             | Corr. |
|----------|---------------------------------------------------------|-------|
| SCCS571  | Resource Base                                           | 0.63  |
| SCCS772  | (No) Litigation                                         | -0.63 |
| SCCS711  | Societal Complexity                                     | 0.62  |
| SCCS1463 | Adults Herd Small Animals                               | 0.62  |
| SCCS835  | Political Integration                                   | 0.6   |
| SCCS883  | Sorcerer/Witch                                          | 0.6   |
| SCCS158  | Scale 10- Social Stratification                         | 0.6   |
| SCCS884  | Priest                                                  | 0.59  |
| SCCS706  | Metalworking                                            | 0.59  |
| SCCS237  | Jurisdictional hierarchy beyond local community         | 0.59  |
| SCCS1130 | Population Density                                      | 0.58  |
| SCCS763  | (Low) Leaders' Exercise of Authority                    | -0.57 |
| SCCS1122 | Log10 of Total Population                               | 0.56  |
| SCCS570  | Fraternal Interest Group Strength                       | 0.56  |
| SCCS762  | (No) Removal of Leaders Who Are Incompetent or Disliked | -0.56 |
| SCCS1738 | Presence of Formal Education within Local Community     | 0.56  |
| SCCS1740 | Levels of Political Hierarchy                           | 0.56  |
| SCCS709  | Social Stratification in the Larger Society             | 0.55  |
| SCCS153  | Scale 5- Technological Specialization                   | 0.55  |
| SCCS1473 | Product Use of Small Animals                            | 0.55  |
| SCCS700  | Crimes against Person Punished                          | 0.54  |
| SCCS89   | Judiciary                                               | 0.54  |
| SCCS1565 | Children hunt with adults                               | -0.54 |
| SCCS699  | Political Organization                                  | 0.54  |
| SCCS756  | (Low) Political Role Differentiation                    | -0.53 |

**Table S2.** Estimated economic and social disparities and gift degree for societies in SCCS. The table shows the ID, several names, latitude, longitude, and estimated values for each society. (Note that IDs of society are different from those of variables even though the same name is used.)

| ID     | Name            | Alternative names                                    | Lat.   | Lon.   | Gift  | Economic | Social |
|--------|-----------------|------------------------------------------------------|--------|--------|-------|----------|--------|
| SCCS1  | Nama            | Khoekhoe, Namaqua, Nama Hottentot                    | -27.5  | 17     | 0.948 | 0.121    | 0.38   |
| SCCS2  | !Kung           | Kung Bushmen, !Kung (Was Nyae), Was Nyae             | -19.83 | 20.58  | 0.395 | 0        | 0      |
| SCCS3  | Tsonga          | Thonga, Tonga, Vatsonga, Bathonga                    | -25.83 | 32.33  | 0.839 | 0.399    | 0.609  |
| SCCS4  | Lozi            | —                                                    | -16    | 23.5   | 0.858 | 0.82     | 0.841  |
| SCCS5  | Mbundu          | Banano, Mbari, Nano, Ovimbundu                       | -12.25 | 16.5   | —     | 1        | 0.731  |
| SCCS6  | Suku            | —                                                    | -6     | 18     | 0.766 | 0.073    | 0.497  |
| SCCS7  | Bemba           | Awemba                                               | -10.5  | 30.5   | —     | 0.414    | 0.715  |
| SCCS8  | Nyakyusa        | —                                                    | -9.5   | 34     | 0.626 | 0.41     | 0.455  |
| SCCS9  | Hadza           | Hadzabe, Hatsa Kindiga, Hadza, Kindiga               | -3.75  | 35.18  | 0.676 | 0.121    | 0.046  |
| SCCS10 | Luguru          | Waluguru                                             | -6.83  | 37.67  | 0.948 | 0.707    | 0.168  |
| SCCS11 | Kikuyu          | Aikikuyu                                             | -0.67  | 37.17  | 0.776 | 0.286    | 0.203  |
| SCCS12 | Ganda           | Baganda                                              | 0.33   | 32.5   | 0.856 | 0.752    | 0.771  |
| SCCS13 | Mbuti           | Sua, BaSua, Kango, BaKango, Bambuti, BaMbuti Pygmies | 1.5    | 28.33  | 0.492 | 0        | 0      |
| SCCS14 | Nkundo          | —                                                    | -0.75  | 19.17  | 0.948 | 0.414    | 0.29   |
| SCCS15 | Banen           | Banyin                                               | 4.67   | 10.8   | 0.966 | 1        | 0.486  |
| SCCS16 | Tiv             | Munshi                                               | 7.25   | 9      | 0.684 | 0.416    | 0.203  |
| SCCS17 | Igbo            | Ibo                                                  | 5.5    | 7.33   | —     | 1        | 0.168  |
| SCCS18 | Fon             | Dahomey, Dahomeans                                   | 7.2    | 1.91   | 0.906 | 0.599    | 0.771  |
| SCCS19 | Ashanti         | Twi                                                  | 7      | -1.5   | 0.865 | 0.507    | 0.609  |
| SCCS20 | Mende           | —                                                    | 7.83   | -12    | 1     | 1        | 0.731  |
| SCCS21 | Wolof           | —                                                    | 13.75  | -15.33 | 0.884 | 0.797    | 0.853  |
| SCCS22 | Bambara         | Bamana                                               | 12.5   | -7     | 0.849 | 0.599    | 0.821  |
| SCCS23 | Tallensi        | —                                                    | 10.66  | -0.57  | 0.619 | 0.583    | 0.658  |
| SCCS24 | Songhai         | —                                                    | 16.58  | -1.67  | 0.966 | 1        | 0.534  |
| SCCS25 | Wodaabe Fulani  | Pastoral Fulani, Wodaabe                             | 15     | 7.5    | 0.584 | 0.706    | 0.258  |
| SCCS26 | Zazzagawa Hausa | Hausa, Zazzagawa                                     | 10.5   | 7.5    | 0.869 | 0.655    | 0.852  |
| SCCS27 | Masa            | Massa                                                | 10.5   | 15.5   | —     | —        | 0.046  |
| SCCS28 | Azande          | Niam-Niam                                            | 5.08   | 28.25  | 0.914 | 0.269    | 0.497  |
| SCCS29 | Fur             | Darfur                                               | 13.5   | 25.5   | 0.845 | 0.526    | 0.609  |
| SCCS30 | Otoro           | Otoro Nuba, Nuba                                     | 11.33  | 30.67  | 0.531 | 0.414    | 0.203  |
| SCCS31 | Shilluk         | —                                                    | 9.75   | 31.5   | 0.573 | 0.799    | 0.959  |
| SCCS32 | Mao             | —                                                    | 9.27   | 34.67  | —     | —        | 0.046  |
| SCCS33 | Kafa            | Kafecho, Kaffa                                       | 7.27   | 36.5   | 0.966 | 1        | 0.837  |

| ID     | Name            | Alternative names    | Lat.  | Lon.   | Gift  | Economic | Social |
|--------|-----------------|----------------------|-------|--------|-------|----------|--------|
| SCCS34 | Maasi           | Masai                | -3.5  | 36.75  | 0.651 | 0.121    | 0.121  |
| SCCS35 | Konso           | —                    | 5.25  | 37.5   | —     | 0.121    | 0.274  |
| SCCS36 | Somali          | —                    | 9     | 47.25  | 0.756 | 0.416    | 0.081  |
| SCCS37 | Amhara          | —                    | 12.5  | 37.75  | 0.878 | 0.816    | 0.852  |
| SCCS38 | Blin            | Bogo, Belen, Bilin   | 15.75 | 38.75  | —     | 1        | 0.756  |
| SCCS39 | Barabra         | Kenuzi Nubians       | 23    | 39.11  | 0.966 | 1        | 0.168  |
| SCCS40 | Teda            | Toubou               | 20.5  | 17.5   | 1     | 0.414    | 0.284  |
| SCCS41 | Tuareg Ahaggar  | Tuareg               | 23    | 6.5    | 0.844 | 0.599    | 0.731  |
| SCCS42 | Riffians        | —                    | 34.92 | -3.25  | 0.876 | 0.56     | 0.274  |
| SCCS43 | Egyptians       | Fellahin, Fellaheen  | 24.75 | 33     | 0.884 | 0.543    | 0.852  |
| SCCS44 | Hebrews         | —                    | 31.18 | 34.92  | —     | 1        | 0.64   |
| SCCS45 | Babylonians     | —                    | 32.58 | 44.75  | 0.385 | 1        | 0.959  |
| SCCS46 | Rwala           | Rwala Bedouin        | 33.25 | 38.5   | 0.885 | 0.752    | 0.587  |
| SCCS47 | Turks           | —                    | 39.33 | 34.25  | 0.826 | 0.616    | 0.959  |
| SCCS48 | Gheg            | Albanians            | 42    | 20.17  | 0.767 | 0.121    | 0.658  |
| SCCS49 | Ancient Romans  | Romans               | 41.67 | 13.5   | —     | 1        | 0.959  |
| SCCS50 | Spanish Basques | Spanish Basques      | 43.25 | -1.67  | 0.826 | 0.459    | 0.959  |
| SCCS51 | Irish           | Gaelic               | 53.5  | -10    | 0.766 | 0.56     | 0.609  |
| SCCS52 | Sami            | Lapps                | 68.7  | 21.5   | 0.53  | 0.121    | 0.081  |
| SCCS53 | Yurak-Samoyeds  | Nenets, Yurak        | 68    | 51.5   | —     | 0.121    | 0.486  |
| SCCS54 | Russians        | —                    | 52.67 | 41.33  | 0.832 | 0        | 0.959  |
| SCCS55 | Abkhaz          | —                    | 43.13 | 40.77  | —     | 1        | 1      |
| SCCS56 | Armenians       | —                    | 40    | 44.5   | —     | 0.121    | 0.959  |
| SCCS57 | Kurd            | —                    | 36.5  | 44.5   | 0.834 | 0.527    | 0.811  |
| SCCS58 | Basseri         | —                    | 29    | 53     | 0.77  | 0.579    | 0.537  |
| SCCS59 | Punjabi         | Punjabi (West)       | 32.5  | 74     | 0.792 | 0.56     | 0.853  |
| SCCS60 | Madia           | Maria Gond, Gond     | 19.63 | 80.92  | 0.821 | 0.121    | 0.395  |
| SCCS61 | Toda            | —                    | 11.5  | 76.5   | 0.8   | 0.379    | 0.258  |
| SCCS62 | Santal          | Santhal, Saontal     | 23.5  | 87.17  | 0.835 | 0.652    | 0.364  |
| SCCS63 | Uttar Pradesh   | —                    | 25.92 | 83     | 0.966 | 0.121    | 0.853  |
| SCCS64 | Burusho         | —                    | 36.43 | 74.58  | 0.677 | —        | 0.973  |
| SCCS65 | Kazakh          | Kazak                | 42.5  | 75.5   | 0.691 | 1        | 0.366  |
| SCCS66 | Khalka          | Xanx, Khalka Mongols | 47.17 | 96.08  | 0.884 | 0.854    | 0.731  |
| SCCS67 | Lolo            | Yi, Nosu             | 27.5  | 103.5  | —     | 1        | 0.412  |
| SCCS68 | Lepcha          | Rong                 | 27.5  | 89     | 0.638 | 0.835    | 0.537  |
| SCCS69 | Garo            | A.Chik               | 26    | 91     | 0.682 | 0.526    | 0.486  |
| SCCS70 | Maras           | Lakher               | 22.33 | 93     | 0.48  | 0.599    | 0.412  |
| SCCS71 | Burmese         | Bamar people         | 22    | 95.67  | 0.569 | 0.782    | 0.853  |
| SCCS72 | Lamet           | —                    | 20    | 100.67 | 0.878 | 0.399    | 0.168  |
| SCCS73 | Annamese        | Vietnamese           | 20.5  | 106.25 | 1     | 0.707    | 0.959  |

| ID      | Name                       | Alternative names                          | Lat.   | Lon.    | Gift  | Economic | Social |
|---------|----------------------------|--------------------------------------------|--------|---------|-------|----------|--------|
| SCCS74  | Rade                       | Rhade                                      | 13     | 108     | —     | 0.121    | 0.168  |
| SCCS75  | Ancient Khmer              | Khmer                                      | 13     | 103.83  | 0.653 | 0.779    | 0.959  |
| SCCS76  | Thai                       | Siamese, Central Thai                      | 14     | 100.85  | —     | 0.121    | 0.959  |
| SCCS77  | Semang                     | —                                          | 5      | 101.25  | 0.332 | 0        | 0.121  |
| SCCS78  | Nicobarese                 | Holchu                                     | 7      | 93.75   | 0.705 | 0.56     | 0.046  |
| SCCS79  | Andamanese                 | Big Andaman Island, Andamense              | 12     | 93      | 0.094 | 0        | 0      |
| SCCS80  | Vedda                      | Wanniyalaeto, Veddah                       | 7.75   | 81.25   | 0.53  | 0        | 0.046  |
| SCCS81  | Tanala                     | —                                          | -22    | 48      | 0.858 | 0.599    | 0.518  |
| SCCS82  | Negri Sembilan             | Negeri Sembilan                            | 2.58   | 102.25  | 1     | 0.121    | 0.715  |
| SCCS83  | Javanese                   | —                                          | -7.7   | 112.22  | —     | 0.121    | 0.959  |
| SCCS84  | Balinese                   | —                                          | -8.5   | 115.33  | 0.983 | 0.121    | 0.852  |
| SCCS85  | Iban                       | Dayak, Sea Dayak                           | 2      | 113     | 0.641 | 0.22     | 0.324  |
| SCCS86  | Badjau Tawi-Tawi           | Tawi-Tawi Badjaw, Badjau                   | 5      | 120     | 0.825 | 0.196    | 0.168  |
| SCCS87  | Toradja                    | —                                          | -2     | 121     | 0.676 | 0.707    | 0.203  |
| SCCS88  | Tobelorese                 | Togutil                                    | 2      | 127.94  | —     | 1        | 0.267  |
| SCCS89  | Alorese                    | Abui                                       | -8.33  | 124.67  | 0.948 | 0.414    | 0.593  |
| SCCS90  | Tiwi                       | —                                          | -11.38 | 131     | 0.398 | 0.216    | 0      |
| SCCS91  | Northern Aranda            | Aranda (Northern), Northern Aranda, Arunta | -24.25 | 133.5   | 0.55  | 0        | 0.046  |
| SCCS92  | Orokaiva                   | —                                          | -8.5   | 148     | 0.159 | 0.196    | 0.121  |
| SCCS93  | Kimam                      | Frederik-Hendrik Islanders                 | -7.5   | 138.5   | —     | 0.121    | 0.046  |
| SCCS94  | Mee                        | Kapauku                                    | -4     | 136     | 0.659 | 0.578    | 0.415  |
| SCCS95  | Kwoma                      | —                                          | -4.17  | 142.67  | 0.8   | 0        | 0.046  |
| SCCS96  | Manus                      | —                                          | -2.17  | 147.17  | 0.66  | 0.121    | 0.203  |
| SCCS97  | Lesu                       | New Irelanders                             | -2.71  | 151     | 0.383 | 0.121    | 0.046  |
| SCCS98  | Trobriands                 | —                                          | -8.54  | 151.01  | 0.509 | 0.312    | 0.284  |
| SCCS99  | Siuai                      | —                                          | -6.76  | 155.45  | 0.385 | 0.121    | 0.168  |
| SCCS100 | Tikopia                    | —                                          | -12.29 | 168.83  | 0.653 | 0.399    | 0.669  |
| SCCS101 | Bunlap                     | Pentecost                                  | -15.95 | 168.22  | —     | 0.121    | 0.168  |
| SCCS102 | Mbau Fijians               | —                                          | -18    | 178.58  | 0.693 | 0.121    | 0.486  |
| SCCS103 | Ajie                       | —                                          | -21.33 | 165.67  | 0.599 | 0.025    | 0.258  |
| SCCS104 | Mori                       | Maori                                      | -35.33 | 174.17  | 0.459 | 0.289    | 0.284  |
| SCCS105 | Marquesans                 | —                                          | -8.92  | -140.17 | 0.384 | 0.121    | 0.29   |
| SCCS106 | Upolu Samoans              | Western Samoans, Upolu                     | -13.94 | -171.77 | 0.53  | 0.121    | 0.477  |
| SCCS107 | Makin                      | Gilbertese                                 | 3.38   | 172.99  | —     | 0.121    | 0.609  |
| SCCS108 | Marshallese (Jaluit Atoll) | —                                          | 6.28   | 169.49  | 0.723 | 0.652    | 0.669  |
| SCCS109 | Trukese                    | Chuukese                                   | 7.34   | 151.6   | 0.709 | 0        | 0.046  |
| SCCS110 | Yapese                     | —                                          | 9.52   | 138.16  | 0.974 | 0.121    | 0.68   |
| SCCS111 | Palauans                   | —                                          | 7.5    | 134.5   | 0.769 | 0.596    | 0.609  |
| SCCS112 | Ifugao                     | —                                          | 16.83  | 121.17  | 0.354 | 1        | 0.203  |

| ID      | Name                   | Alternative names                                                                                              | Lat.  | Lon.    | Gift  | Economic | Social |
|---------|------------------------|----------------------------------------------------------------------------------------------------------------|-------|---------|-------|----------|--------|
| SCCS113 | Atayal                 | —                                                                                                              | 24.33 | 120.75  | —     | 0.414    | 0.046  |
| SCCS114 | Chekiang               | Chinese                                                                                                        | 31    | 120.08  | 0.861 | 0.634    | 0.959  |
| SCCS115 | Manchu                 | —                                                                                                              | 50    | 125.5   | —     | 0.414    | 0.168  |
| SCCS116 | Koreans                | —                                                                                                              | 37.6  | 126.42  | 0.867 | 0.854    | 0.973  |
| SCCS117 | Japanese               | —                                                                                                              | 34.67 | 133.67  | 0.884 | 0.459    | 0.853  |
| SCCS118 | Ainu                   | Ainu (Hokkaido), Hokkaido                                                                                      | 42.83 | 143     | 0.625 | 0.121    | 0.243  |
| SCCS119 | Nivkh                  | Gilyak                                                                                                         | 53    | 142     | 0.685 | 0.379    | 0      |
| SCCS120 | Yukaghir               | —                                                                                                              | 64.75 | 153.5   | 0.095 | 0.414    | 0.046  |
| SCCS121 | Chukchi                | Iygoravetlyan, Ankalyan, Chavchu, Chukchee                                                                     | 66.5  | 179.6   | 0.595 | 0.509    | 0.168  |
| SCCS122 | Deg Xit'an             | Ingalik                                                                                                        | 62.5  | -159.5  | 0.622 | 0.617    | 0.081  |
| SCCS123 | Aleut                  | Unagan                                                                                                         | 55    | -162.85 | 0.545 | 0.779    | 0.731  |
| SCCS124 | Copper Inuit           | Kitlinermiut, Copper Eskimo                                                                                    | 68.72 | -112.53 | 0.368 | 0.121    | 0      |
| SCCS125 | Montagnais             | Innu, Naskapi                                                                                                  | 50    | -74     | 0.479 | 0        | 0.046  |
| SCCS126 | Mi'kmaq                | Micmac                                                                                                         | 46.99 | -65     | 0.529 | 0.121    | 0.046  |
| SCCS127 | Northern Saulteaux     | N. Saulteaux, North Saulteaux                                                                                  | 52    | -95.5   | 0.368 | 0.121    | 0      |
| SCCS128 | DeneTha                | Slave, Deh Cho (Southern Slavey), Slavey, Dene (distinguish from speakers of the Dene language)                | 62    | -122    | 0.354 | 0.121    | 0      |
| SCCS129 | Kaska                  | Nahane                                                                                                         | 60    | -131    | 0.587 | 0.459    | 0.046  |
| SCCS130 | Eyak                   | dAXunhyuu                                                                                                      | 60.5  | -145    | 0.649 | 0.452    | 0.415  |
| SCCS131 | Haida                  | —                                                                                                              | 54    | -132.5  | —     | 1        | 0.412  |
| SCCS132 | Nuxalk                 | Nuxalkmc, Bellacoola, Bilqula, Bella Coola                                                                     | 52.33 | -126.5  | 0.826 | 0.852    | 0.366  |
| SCCS133 | Twana                  | —                                                                                                              | 47.43 | -123.25 | 0.547 | 0.618    | 0.168  |
| SCCS134 | Yurok                  | —                                                                                                              | 41.5  | -124    | 0.537 | 0.651    | 0.168  |
| SCCS135 | Eastern Pomo           | Clear Lake Pomo, Eastern Pomo                                                                                  | 39    | -123    | 0.776 | 0.399    | 0.168  |
| SCCS136 | Southern Valley Yokuts | Lake Yokuts, Tachi Yokuts, Chunut Yokuts                                                                       | 35    | -119.5  | 0.652 | 0.183    | 0.415  |
| SCCS137 | Wadadokado             | Paiute, Northern Paiute                                                                                        | 43.5  | -119    | 0.383 | 0.121    | 0.046  |
| SCCS138 | Klamath                | —                                                                                                              | 42.63 | -121.67 | 0.659 | 0.414    | 0.446  |
| SCCS139 | Kutenai                | Ktunaxa, Kootenay, Kootenai                                                                                    | 49    | -116.67 | 0.518 | 0.49     | 0.046  |
| SCCS140 | Gros Ventre            | A'ani, A'aninin, Haaninin                                                                                      | 48    | -108    | 0.354 | 0.121    | 0.121  |
| SCCS141 | Hidatsa                | —                                                                                                              | 47    | -101    | 0.679 | 0.121    | 0.046  |
| SCCS142 | Pawnee                 | —                                                                                                              | 42    | -100    | 0.607 | 0.471    | 0.29   |
| SCCS143 | Omaha                  | Dhegiha                                                                                                        | 41.43 | -96.5   | —     | 0.414    | 0.046  |
| SCCS144 | Huron                  | Bear and Cord Peoples, Wendat, Ouendat, Attignauquantan, Attinniaonten, Attigneonongnahac, Hatingeennonniyahak | 44.5  | -79     | 0.652 | 0.379    | 0.537  |
| SCCS145 | Muscogee               | Creek, Taskigi Creek                                                                                           | 32.93 | -86     | 0.825 | 0.36     | 0.046  |

| ID      | Name               | Alternative names                                                      | Lat.   | Lon.    | Gift  | Economic | Social |
|---------|--------------------|------------------------------------------------------------------------|--------|---------|-------|----------|--------|
| SCCS146 | Natchez            | —                                                                      | 31.5   | -91.42  | 0.948 | —        | 0.731  |
| SCCS147 | Comanche           | —                                                                      | 34     | -101.5  | 0.525 | 0.472    | 0.121  |
| SCCS148 | Chiricahua         | Chiricahua Apache, Eastern Apache                                      | 32     | -109.5  | 0.368 | 0.121    | 0.334  |
| SCCS149 | Zuni               | —                                                                      | 35.67  | -108.75 | 0.825 | 0.025    | 0.046  |
| SCCS150 | Havasupai          | Plateau Yuma                                                           | 35.83  | -112.17 | 0.485 | 0.121    | 0      |
| SCCS151 | Tohono O’odham     | Papago                                                                 | 32     | -112    | 0.53  | 0.121    | 0      |
| SCCS152 | Huichol            | Wixárika                                                               | 22     | -105    | —     | 0.121    | 0.168  |
| SCCS153 | Aztec              | Aztec of Tenochtitlan                                                  | 19     | -99.17  | 0.907 | 0.69     | 0.781  |
| SCCS154 | Sierra Popoluca    | Popoluca, Soteapanec Zoque, Soteapan Zoque, Soteapaneco, Soteapan Soke | 18.25  | -94.83  | —     | 0.121    | 0.364  |
| SCCS155 | K’iche’            | Quiche                                                                 | 15     | -91     | —     | 1        | 0.593  |
| SCCS156 | Miskito            | Mískitu, Mosquito                                                      | 15     | -83     | 0.674 | 0        | 0.046  |
| SCCS157 | Bribri             | Talamanca                                                              | 9      | -83.25  | 0.383 | 0.121    | 0.046  |
| SCCS158 | Guna               | Dule, Tule, Cuna, Kuna                                                 | 9.25   | -78.5   | 0.53  | 0.707    | 0.537  |
| SCCS159 | Wayuu              | Goajiro                                                                | 11.92  | -71.75  | 0.673 | 0.799    | 0.345  |
| SCCS160 | Haitians           | —                                                                      | 18.83  | -72.17  | 0.857 | 0.835    | 0.959  |
| SCCS161 | Callinago          | —                                                                      | 15.41  | -61.27  | 0.383 | 1        | 0.168  |
| SCCS162 | Warao              | Warrau                                                                 | 9.08   | -62     | 0.676 | 0.121    | 0.471  |
| SCCS163 | Yanomami           | Yanomamo, Yanoama                                                      | 2.42   | -65     | 0.479 | 0        | 0.046  |
| SCCS164 | Barama River Carib | Barama Carib, Carib                                                    | 7.42   | -60.17  | 0.368 | 0.121    | 0.121  |
| SCCS165 | Saramaccană        | Saramaccan of Suriname, Saramacca, Bush Negroes                        | 3.5    | -55.75  | 0.573 | 0        | 0.364  |
| SCCS166 | Munduruku          | Wuy Jugu, Mundurucu                                                    | -6.5   | -56.5   | 0.342 | 0        | 0.121  |
| SCCS167 | Cubeo              | Jiwa, Tucano                                                           | 1.25   | -70.5   | 0.644 | 0.22     | 0.168  |
| SCCS168 | Chachi             | Cayapa                                                                 | 1      | -79     | 0.66  | 0.121    | 0.121  |
| SCCS169 | Shuar              | Jivaro                                                                 | -3     | -78     | 0.534 | 0        | 0      |
| SCCS170 | Amahuaca           | —                                                                      | -10.33 | -72.25  | —     | 0.121    | 0.046  |
| SCCS171 | Inca               | —                                                                      | -13.5  | -72     | 0.676 | 0.121    | 0.959  |
| SCCS172 | Aymara             | —                                                                      | -16    | -65.75  | 0.893 | 0.579    | 0.168  |
| SCCS173 | Sirionó            | Miá, Siriono                                                           | -14.5  | -63.5   | 0     | 0        | 0.046  |
| SCCS174 | Nambikwara         | Nambicura                                                              | -13    | -58.75  | 0.374 | 0.121    | 0.121  |
| SCCS175 | Trumai             | Ho kod ke                                                              | -11.83 | -53.67  | 0.644 | 0.073    | 0.046  |
| SCCS176 | Canela             | Ramcocamecra, Timbira, Canella                                         | -6.5   | -46     | 0.433 | 0        | 0.121  |
| SCCS177 | Tupinambá          | Tupinamba                                                              | -22.79 | -44.5   | 0.239 | 0.414    | 0.168  |
| SCCS178 | Aimoré             | Nac-nanuk, Nac-poruk, Botocudo                                         | -19    | -42.5   | —     | 0.121    | 0.046  |
| SCCS179 | Shavante           | —                                                                      | -13.5  | -51.5   | 0.264 | 0        | 0      |

| ID      | Name      | Alternative names                                                                                                                                | Lat.  | Lon.   | Gift  | Economic | Social |
|---------|-----------|--------------------------------------------------------------------------------------------------------------------------------------------------|-------|--------|-------|----------|--------|
| SCCS180 | Aweikoma  | Xokleng, Shokleng, Botocudo of Santa Catarina, Bugre, Kaingang of Santa Catarina (though Aweikoma and Kaingang today considered separate groups) | -28   | -50    | 0.166 | 0        | 0      |
| SCCS181 | Cayua     | Abá, Cayua, Caingua, Guaraní, Guarani                                                                                                            | -23.5 | -55    | —     | —        | 0.046  |
| SCCS182 | Lengua    | —                                                                                                                                                | -23   | -58.5  | 0.383 | 0.121    | 0.046  |
| SCCS183 | Abipón    | Abipon, Abipones                                                                                                                                 | -28   | -59.5  | 0.369 | 1        | 0.366  |
| SCCS184 | Mapuche   | —                                                                                                                                                | -38.5 | -72.58 | 0.682 | 0.472    | 0.608  |
| SCCS185 | Tehuelche | Patagon                                                                                                                                          | -40.5 | -68    | —     | 0.414    | 0.046  |
| SCCS186 | Yahgan    | —                                                                                                                                                | -55.5 | -69.5  | 0.623 | 0        | 0      |

## **Values of SCCS Variables Used for Data Analyses**

The values of SCCS variables are explained as below, according to [1, 2]

### **SCCS89 Judiciary**

1. Absent, 2. Not local, 3. Executive, 4. Appointed by executive, 5. Priesthood, and 6. Hereditary.

### **SCCS91 Administrative Hierarchy**

1. Absent, 2. Popular Assemblies, 3. Heads of kin groups, 4. Heads of decentralized territorial divisions, 5. Heads of centralized territorial divisions, and 6. Part of centralized system.

### **SCCS153 Technological Specialization**

1. None, 2. Pottery only, 3. Loom weaving only, 4. Metalwork only, and 5. Smiths, weavers, potters.

### **SCCS158 Social Stratification**

1. Egalitarian, 2. Hereditary slavery, 3. 2 social classes, no castes/slavery, 4. 2 social classes, castes/slavery, and 5. 3 social classes or castes, with or without slavery.

### **SCCS237 Jurisdictional hierarchy beyond local community**

1. No political authority beyond community (e.g., autonomous bands and villages), 2. One level (e.g., petty chiefdoms), 3. Two levels (e.g., larger chiefdoms), 4. Three levels (e.g., states), and 5. Four levels (e.g., large states).

### **SCCS568 Compensation Demands**

1. Absent and 2. Present

### **SCCS570 Fraternal Interest Group Strength**

1. Both brideprice and patrilineality are absent, and size of effective kin-based political subunit is less than 100, 2. Either brideprice or patrilineality; size of political subunit between 100 and 999, 3. a. Size of political subunit is 1,000 or greater, and brideprice and patrilineality are absent; or b. Size of political subunit is less than 100 and both brideprice and patrilineality are present; or c. Size of political subunit is between 100 and 999 and either brideprice or patrilineality is present, 4. a. Size of political subunit is between 100 and 999, and both brideprice and patrilineality are present; or b. Size of political subunit is 1,000 or greater, and either brideprice or patrilineality is present, and 5. Size of political subunit is 1,000 or greater, and both brideprice and patrilineality are present.

### **SCCS571 Resource Base**

1. Low, 2. Unstable, and 3. High.

### **SCCS699 Political Organization (Adapted from Murdock 1961, P. 207)**

1. Absence of local political integration - family heads acknowledge no higher authority, 2. Autonomous local community - population below 1500, 3. Minimal State - political integration in independent units averaging 1500 - 10,000, 4. Little State - political integration in independent units averaging 10,000 - 100,000, and 5. State political integration in a unit of 100,000.

### **SCCS700 Crimes against Person Punished**

1. By person or group wronged and 2. By government action.

### **SCCS706 Metalworking**

0. Absent, and 1. Present.

### **SCCS709 Social Stratification in the Larger Society**

1. Lack of significant stratification among free men, 2. Differences in wealth and control, but not crystallized into distinct and hereditary social classes, 3. Dual stratification into hereditary elites and commoners, and 4. Complex stratification into three or more classes/castes.

### **SCCS711 Societal Complexity (Guttman Scale - Freeman and Winch 1957)**

1. Absence of all traits in scale, 2. Crimes punished by government, 3. Full-time specialized priests, 4. Formal education, 5. Written language, and 6. Full-time bureaucrats.

### **SCCS756 (Low) Political Role Differentiation: Full Time Specialists and Their Differentiation from Others in the Society**

1. Highly differentiated by wealth, special titles or life style, 2. Moderately differentiated, 3. Somewhat wealthier but share much of life style by age, gender, 4. Same life style, may be older and have somewhat more prestige, 5. Few exist but leadership roles present, wealthier than others, 6. Few exist but leadership roles present, same life style, and 7. None exist, no permanent leadership roles.

### **SCCS762 (No) Removal of Leaders Who Are Incompetent or Disliked**

1. No way other than rebellion or popular uprisings, 2. Institutionalized means invoked occasionally, possibly by elites, 3. Not removed in formal manner but lose influence and are ignored, and 4. No formal leadership, loss of power when support diminishes.

**SCCS763 (Low) Leaders' Exercise of Authority**

1. Frequently act independently and make authoritative decisions, 2. Make relatively few decisions on own without consultation, and 3. Use persuasion to help organized and structure group action.

**SCCS772 (No) Litigation: Use of Third Parties Offering Binding Decisions, with or without Formal Court Systems**

1. Frequent involvement in litigation by society members, 2. Occasional involvement, and 3. Rare or non-involvement.

**SCCS784 (No) Taxation Paid to Community (e.g., in Agricultural Produce, Labour, Finished Goods)**

1. Regular and non-negligible taxes to community, 2. Only in special situations or Modest level, and 3. None.

**SCCS835 Political Integration**

1. Independent local communities, 2. Single level of political integration, 3. Two levels of supra-community integration, and 4. Three or more levels of supra-community integration.

**SCCS883 Sorcerer/Witch**

0. Absent, and 1. Present.

**SCCS884 Priest**

0. Absent, and 1. Present.

**SCCS973 Degree of Marriage Celebration**

1. There is no celebration, 2. There is a small celebration, e.g., a minor acknowledgement or exchange of gifts, 3. There is a moderate celebration, e.g., a feast, dancing, dramatic performances, or extensive gift exchange, and 4. There is an elaborate celebration, e.g., it lasts a long period of time, is characterized by lavish dress, has elaborate performances, etc.

**SCCS1122 Log10 of Total Population**

- Log10 of Total Population

**SCCS1130 Population Density (from Pryor Data)**

2. less than 1 per square mile, 3. 1 - 4.9 per square mile, 4. 5 - 24.9 per square mile, 5. 25 - 99.9 per square mile, 6. 99 - 499.9 per square mile, and 7. 500 or more per square mile.

**SCCS1463 Adults Herd Small Animals**

0. Activity not present, 1. Men Only, 2. Men Predominant, 5. Women Only, 6. Not an Adult Task, and 10. Slaves Only.

**SCCS1473 Product Use of Small Animals**

0. None (e.g., activity not present), 2. Product consumer is household or community, 4. Household and wage labor or product sold, and 5. 1 and 2 above.

**SCCS1565 Children hunt with adults**

0. Activity not present, 1. Yes, Children do this, and 2. No, Children do not do this.

**SCCS1721 Number of Rich People (Wealthy)**

10. Absence of rich, 20. Presence of rich, no information on numbers, 21. Few rich, and 22. Many rich.

**SCCS1723 Number of Poor**

10. Absence of poor, 20. Presence of poor, no information on numbers, 21. Few poor, and 22. Many poor.

**SCCS1724 Number of Dispossessed**

10. Absence of dispossessed, 20. Presence of dispossessed, no information on numbers, 21. Few dispossessed, and 22. Many dispossessed.

**SCCS1733 Market Exchange within Local Community**

10. No market exchange, 20. Market exchange within local community present, no further information, 21. Market exchange within local community present, involving local and regional products, and 22. Market exchange within local community present, involving local, regional, and supra-regional products.

**SCCS1736 Tribute, Taxation, Expropriation**

10. No tribute, taxation, or expropriation, 20. Payment of tribute, taxation, or expropriation occur, 21. Corvéé labor, 22. Money, 23. Mobile goods, and 24. More than one of the above.

**SCCS1738 Presence of Formal Education within Local Community**

10. No formal education, 20. Formal education present, 21. Small fraction of local community is formally educated, 22. Large part of local community is formally educated, and 23. Members of local community have a higher education.

**SCCS1740 *Levels of Political Hierarchy***

10. No political office, 20. No political office at the head of local community, but segments of different local communities belong to supralocal non-territorially organized political unit, 21. Highest political office one level above smallest supralocal non-territorially organized political unit, 22. Highest political office two levels above smallest supralocal non-territorially organized political unit, 23. Highest political office three levels above smallest supralocal non-territorially organized political unit, 24. Highest political office four levels above smallest supralocal non-territorially organized political unit, 30. Highest political office at the head of local community (=politically autonomous local community), 31. Highest political office one level above local community, 32. Highest political office two levels above local community, 33. Highest political office three levels above local community, and 34. Highest political office four or more levels above local community.

**SCCS1741 *Overarching Formal Jurisdiction within Unit of Maximal Political Authority***

1. No formal jurisdiction present, 2. Highest level of formal jurisdiction below the unit of maximal political authority, and 3. Highest level of formal jurisdiction at the level of maximal political authority.

**REFERENCES**

1. G. P. Murdock and D. R. White, "Standard cross-cultural sample," *Ethnology* **8**, 329–369 (1969).
2. K. R. Kirby, R. D. Gray, S. J. Greenhill, F. M. Jordan, S. Gomes-Ng, H.-J. Bibiko, D. E. Blasi, C. A. Botero, C. Bowern, C. R. Ember *et al.*, "D-place: A global database of cultural, linguistic and environmental diversity," *PloS one* **11**, e0158391 (2016).
